# Supplementary material for: Ferromagnetic resonance response in square artificial spin ice: roles of geometry in vertex dynamics and magnetic configurations
Source: arXiv:2405.01720 source file (2024-06-28)
Supplement: Supplementary file 1 [file Suplementar.pdf]

# Ferromagnetic resonance response in square artificial spin ice: roles of geometry in vertex dynamics and magnetic configurations
Supplementary Information

## S1. FMR response as function of $H^{\text{bias}}$ applied along the easy axis

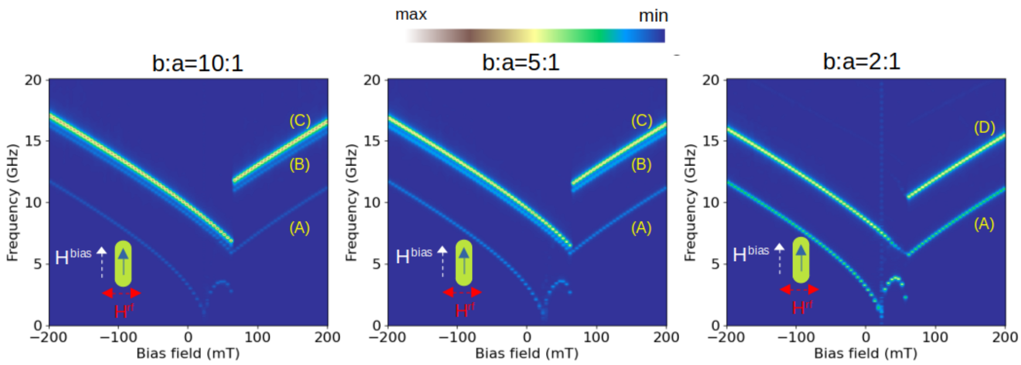


Figure S1: Broadband FMR spectra of individual nanoisland when $H^{\text{bias}}$ applied along easy axis, according to the the aspect ratio $b$:$a$=1:10 , $b$:$a$=1:5, and $b$:$a$=1:2.

Figure S1 displays the simulated broadband FMR of an individual nanoisland when $H^{\text{bias}}$ is applied along the easy axis. The resonance branch (A) is related to the short edge mode, branch lines (B) correspond to the higher-order mode from (A) resonance mode, and branch (C) corresponds to the bulk mode. The branch (B) and (C) is clearly defined for the aspect ratios $a$:$b$=1:10 and $a$:$b$=1:5. However, when $a$:$b$=1:2, these resonance branches overlap and appear a new resonance mode represented by the branch (D).

## S2. FMR response as function of $H^{\text{bias}}$ applied along the hard axis

Figure S2 displays the simulated broadband FMR of an individual nanoisland with $H^{\text{bias}}$ applied along the hard axis. The region 1 corresponds to the saturated state along the hard axis. The broadband FMR shows two regions (1 and 2). Region 1 corresponds to the saturated state with the following branches corresponding to oscillation modes: branches (E), representing the main resonance mode, and (F) higher-order resonances modes; the branch (G) corresponds to resonance modes from a combination of short-edge and long-edge modes; the branch (H) indicates bulk oscillation modes. As the aspect ratio decreases, region 1 widens with gradually reducing high-order modes (F). Region 2 displays the resonance modes in the non-saturated

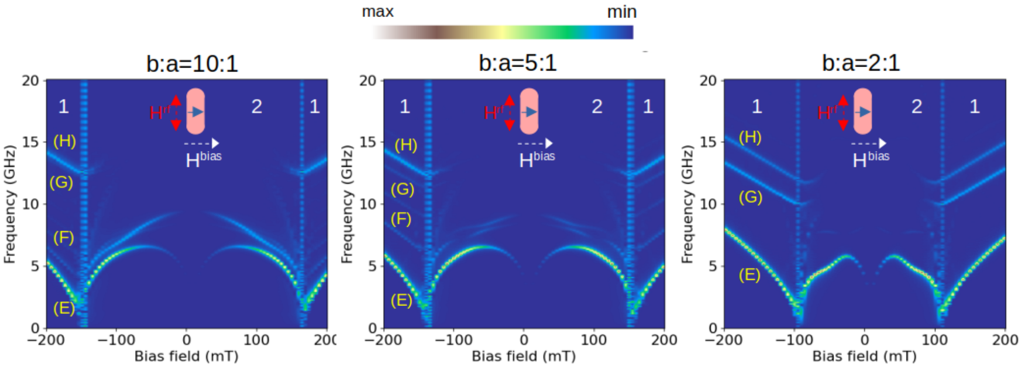


Figure S2: Broadband FMR spectra of individual nanoisland when $H^{\text{bias}}$ applied along hard axis, according to the the aspect ratio *b*:*a*=1:10 , *b*:*a*=5:1, and *b*:*a*=2:1.

states, negligible at the remanence ($H^{\text{bias}} = 0$) due to the equilibrium magnetization aligning along the long axis of the nanoislands. The boundaries of region 2 are contingent upon the aspect ratio, dictated by the minimum saturated field: at an aspect ratio of $b : a = 10 : 1$, it stands at |163| mT; for $b : a = 5 : 1$, it resides at |155| mT; at $b : a = 3 : 1$, it lies at |125| mT; and for $b : a = 2 : 1$, it rests at |110| mT.

## S3. FMR response as function of $H^{\text{bias}}$ applied along the hard axis, with $H^{\text{bias}}$ parallel to $H^{\text{rf}}$ field.

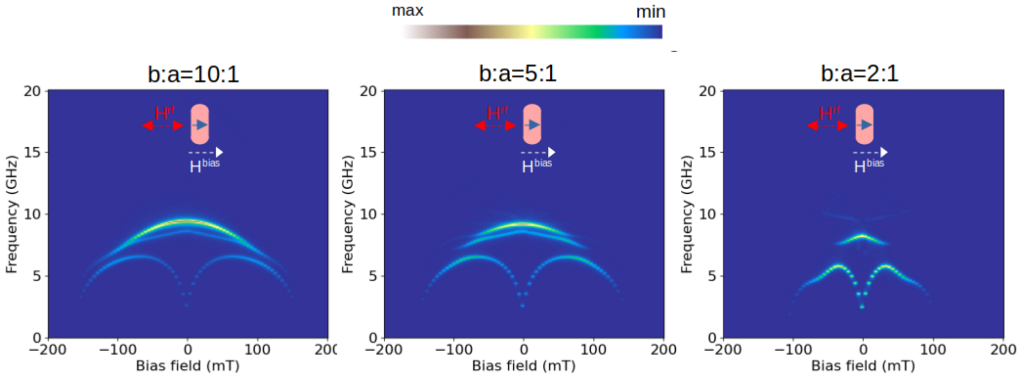


Figure S3: Simulated broadband FMR spectra of individual nanoisland when $H^{\text{bias}}$ is applied along hard axis and parallel $H^{\text{rf}}$ according to the aspect ratio: a) *a:b*=1:10 , b) *a:b*=1:5, c) *a:b*=1:2.

Figure S3 shows the simulated broadband FMR characteristics of an individual nanoisland with $H^{\text{bias}}$ applied along the hard axis but parallel to $H^{\text{rf}}$, which permits excite resonance at the remanence ($H^{\text{bias}} = 0$). Only region 2 appears in this case, and the resonance modes in the remanence are discernible due to the magnetization in the nanoisland lying in the long axis, making appreciable $H^{\text{rf}}$ stimulation. At the remanence state, for all aspect ratios, the FMR response results similar to the FMR response when $H^{\text{bias}}$ lies along the easy axis.

## S4. Ferromagnetic resonance in one ASI vertex saturated according to the aspect ratio.

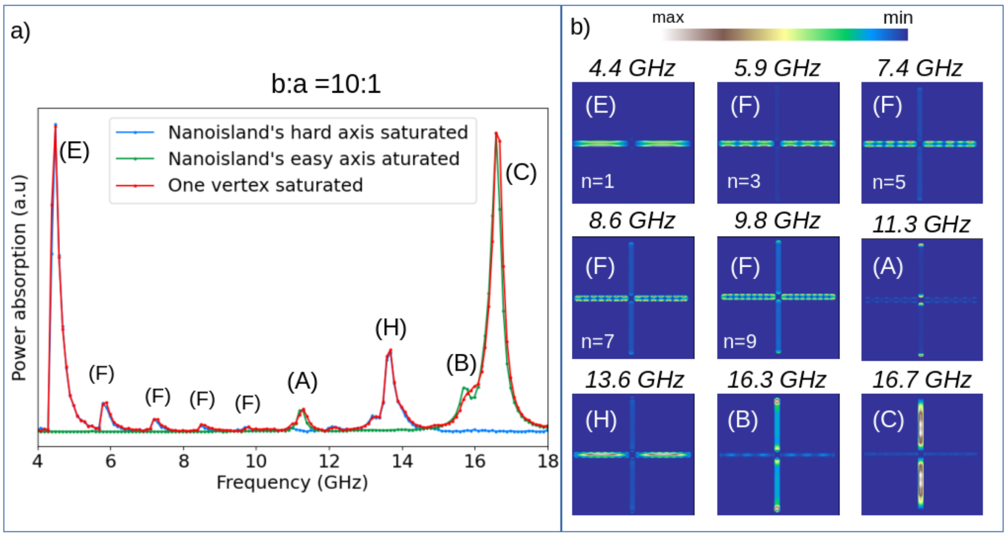


Figure S4-1: Ferromagnetic resonance in one square ASI vertex saturated according to the aspect ratio $b$:$a$=10:1: a) FMR spectra b) Spatial profiles modes

Figure S4-1(a) shows the ferromagnetic resonance when the aspect ratio is $b$:$a$=10:1 in a saturated ASI vertex, compared with FMR spectra of individual nanoislands; and figure S4-1(b) shows the spatial profiles modes. The FMR spectra show the splitting of FMR frequencies into horizontal or vertical nanoislands, which denote oscillation modes into the hard and easy axes. The matching of the FMR spectra with the FMR response from individual nanoislands and spatial profile modes corroborates this. Resonance peak modes (E) at 4.4 GHz are related to the main resonance mode ($n$ = 1) from the long edge of the horizontal nanoislands. The peaks (F) correspond to their higher-order resonance modes with odd harmonics number $n = \{3, 5, 7, 9\}$. The peaks (A) correspond to the short edges resonance modes, unaffected by the aspect ratio due to the fixed short axis $a$, and with high order resonance mode in the peak (B). The peaks (H) and (C) correspond to bulk modes from horizontal and vertical nanoislands respectively.

Figure S4-2 shows the ferromagnetic resonance in a saturated ASI vertex for aspect ratio is $b$:$a$=5:1. Figure S4-2(a) exhibits the FMR response from one ASI vertex compared with the FMR response from individual nanoisland with $H^{\text{bias}}$ applied along the hard and easy axes, revealing slightly mismatch of one ASI vertex due to the presence of dipolar fields between the nanoislands. Additionally, figure S4-2(b) exhibits the spatial profile modes of one saturated vertex, which reveals the splitting of FMR response between horizontal and vertical nanoislands. Power absorption with resonance peaks (E) at 5.1 GHZ is related to the main resonance mode of the long edges from horizontal nanoislands. Higher-order resonance modes (F) reduce to two odd harmonics ($n = \{3, 5\}$). Resonance peak (A) with frequency at 11.3 GHz corresponds to the short-edge modes, with their high-order resonance (B) at 15.7 GHz. Peaks (G) are a combination of long-edge and short-edge resonance modes. The peaks (H) and (C) are bulk modes from horizontal and vertical nanoislands.

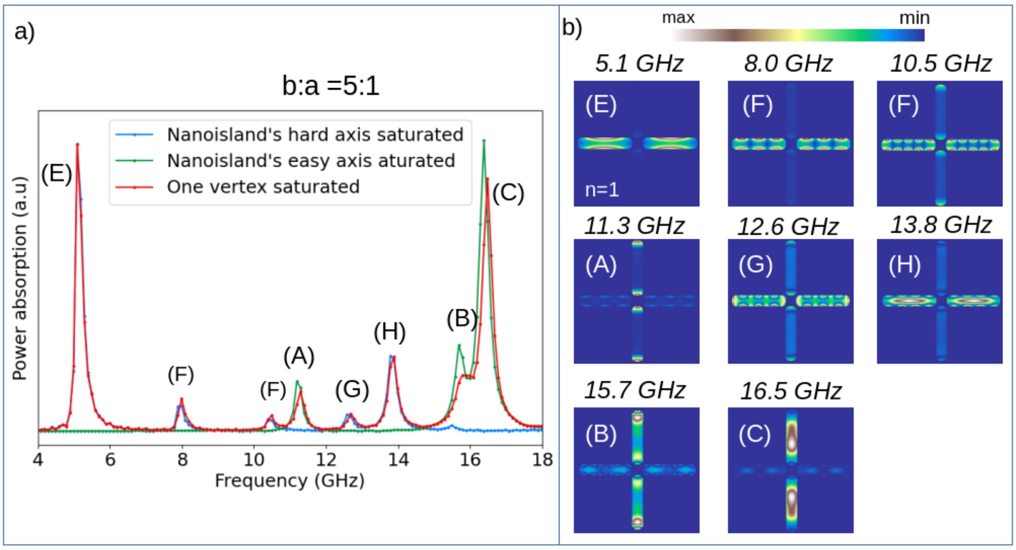


Figure S4-2: Ferromagnetic resonance in one square ASI vertex saturated according to the aspect ratio $b$:$a$=5:1: a) FMR spectra b) Spatial profiles modes

Figure S4-3 shows the ferromagnetic resonance for the aspect ratio $b$:$a$=2:1 in one square ASI vertex. Similarly, for the other aspect ratios, figure S4-3(a) displays the FMR spectra compared with the FMR spectra of individual nanoislands. As expected, frequencies are splitting into horizontal or vertical nanoisland, which denotes oscillations into the hard and easy axes. The slightly mismatched ASI vertex, observed for the highest aspect ratios, increases for b:a=2:1, denoting higher dipolar fields between the nanoislands.

Resonance peaks (E) at 7.4 GHZ exhibit the main resonance mode of the long edge from horizontal nanoislands. The Resonance peak (A) with a fixed frequency at 11.3 GHz corresponds to the short-edges modes, with their high-order resonance (B) at 15.7 GHz. The peaks (G) combine long-edge and short-edge resonance modes. The peaks (H) and (D) are bulk modes from horizontal and vertical nanoislands respectively. The peaks (D) reveal a hybridization and overlapping from bulk modes (C) and higher-order resonance modes (E) exposed in the other aspect ratios.

## S5. Spatial profiles of the in-plane magnetization oscillations, in quadrature with $H^{\mathrm{rf}}$ at Vertex in Square ASI lattice for aspect ratio 5:1.

Figure S5 exhibits the spatial profile of magnetization from oscillation modes in (V) and (W) peaks in the remanent state, in quadrature with $H^{\mathrm{rf}}$. The figure highlights in-phase and out-of-phase modes for the Type III_2 states in bulk modes (W). The oscillation modes in phase exhibit the same color in the figure, while oscillation modes out of phase have different colors, representing almost a phase of $\pi$ degrees for type III_2 at 9.3 GHz.

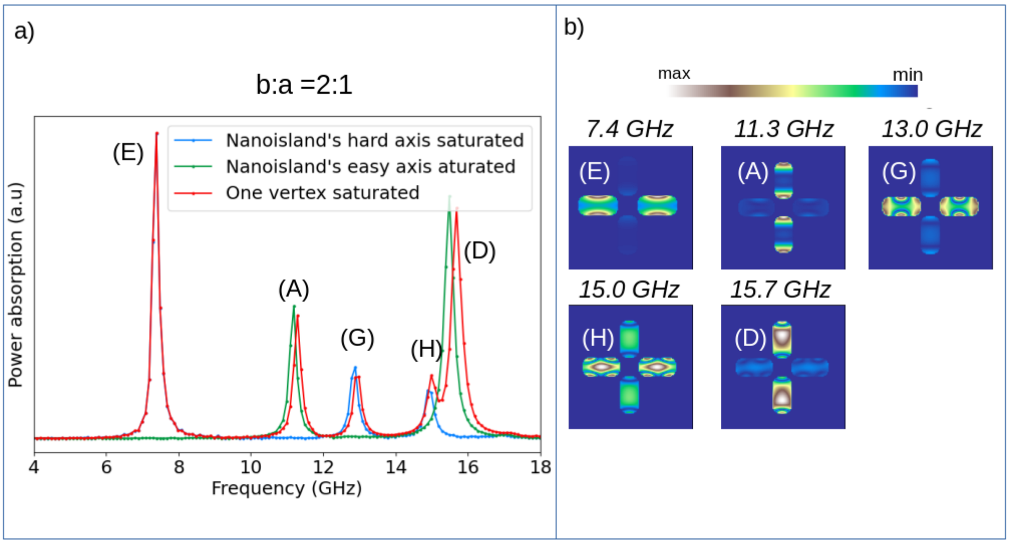


Figure S4-3: Ferromagnetic resonance in one square ASI vertex saturated according to the aspect ratio *b*:*a*=1:2: a) FMR spectra b) Spatial profiles modes

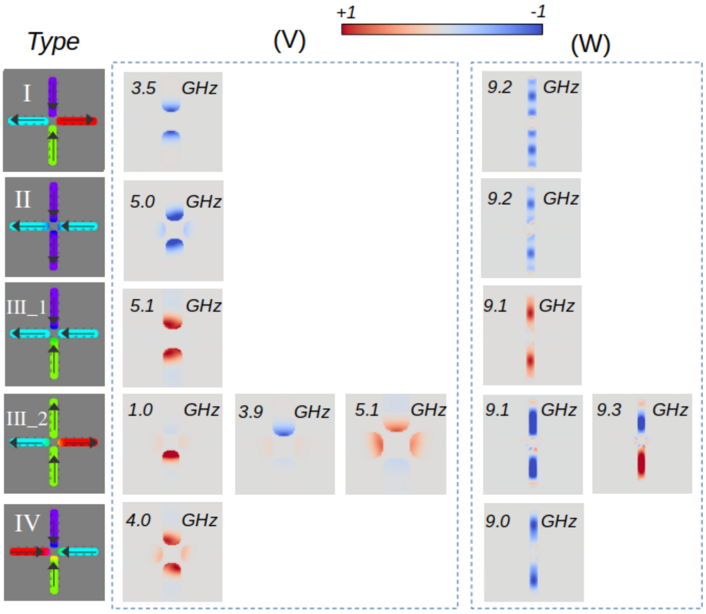


Figure S5: Spatial profiles of the in-plane magnetization oscillations, in quadrature with $H^{\mathrm{rf}}$, at vertex in a square ASI lattice for aspect ratio 5:1, according to energy state.
